# Supplementary material for: WDNet: Watermark-Decomposition Network for Visible Watermark Removal
Source: arXiv:2012.07616 source file (2020-12-15)
Supplement: Supplementary file 2 [file fig_sup_ablation.tex]

\begin{figure*}[h]
\centering
\includegraphics[width=\linewidth]{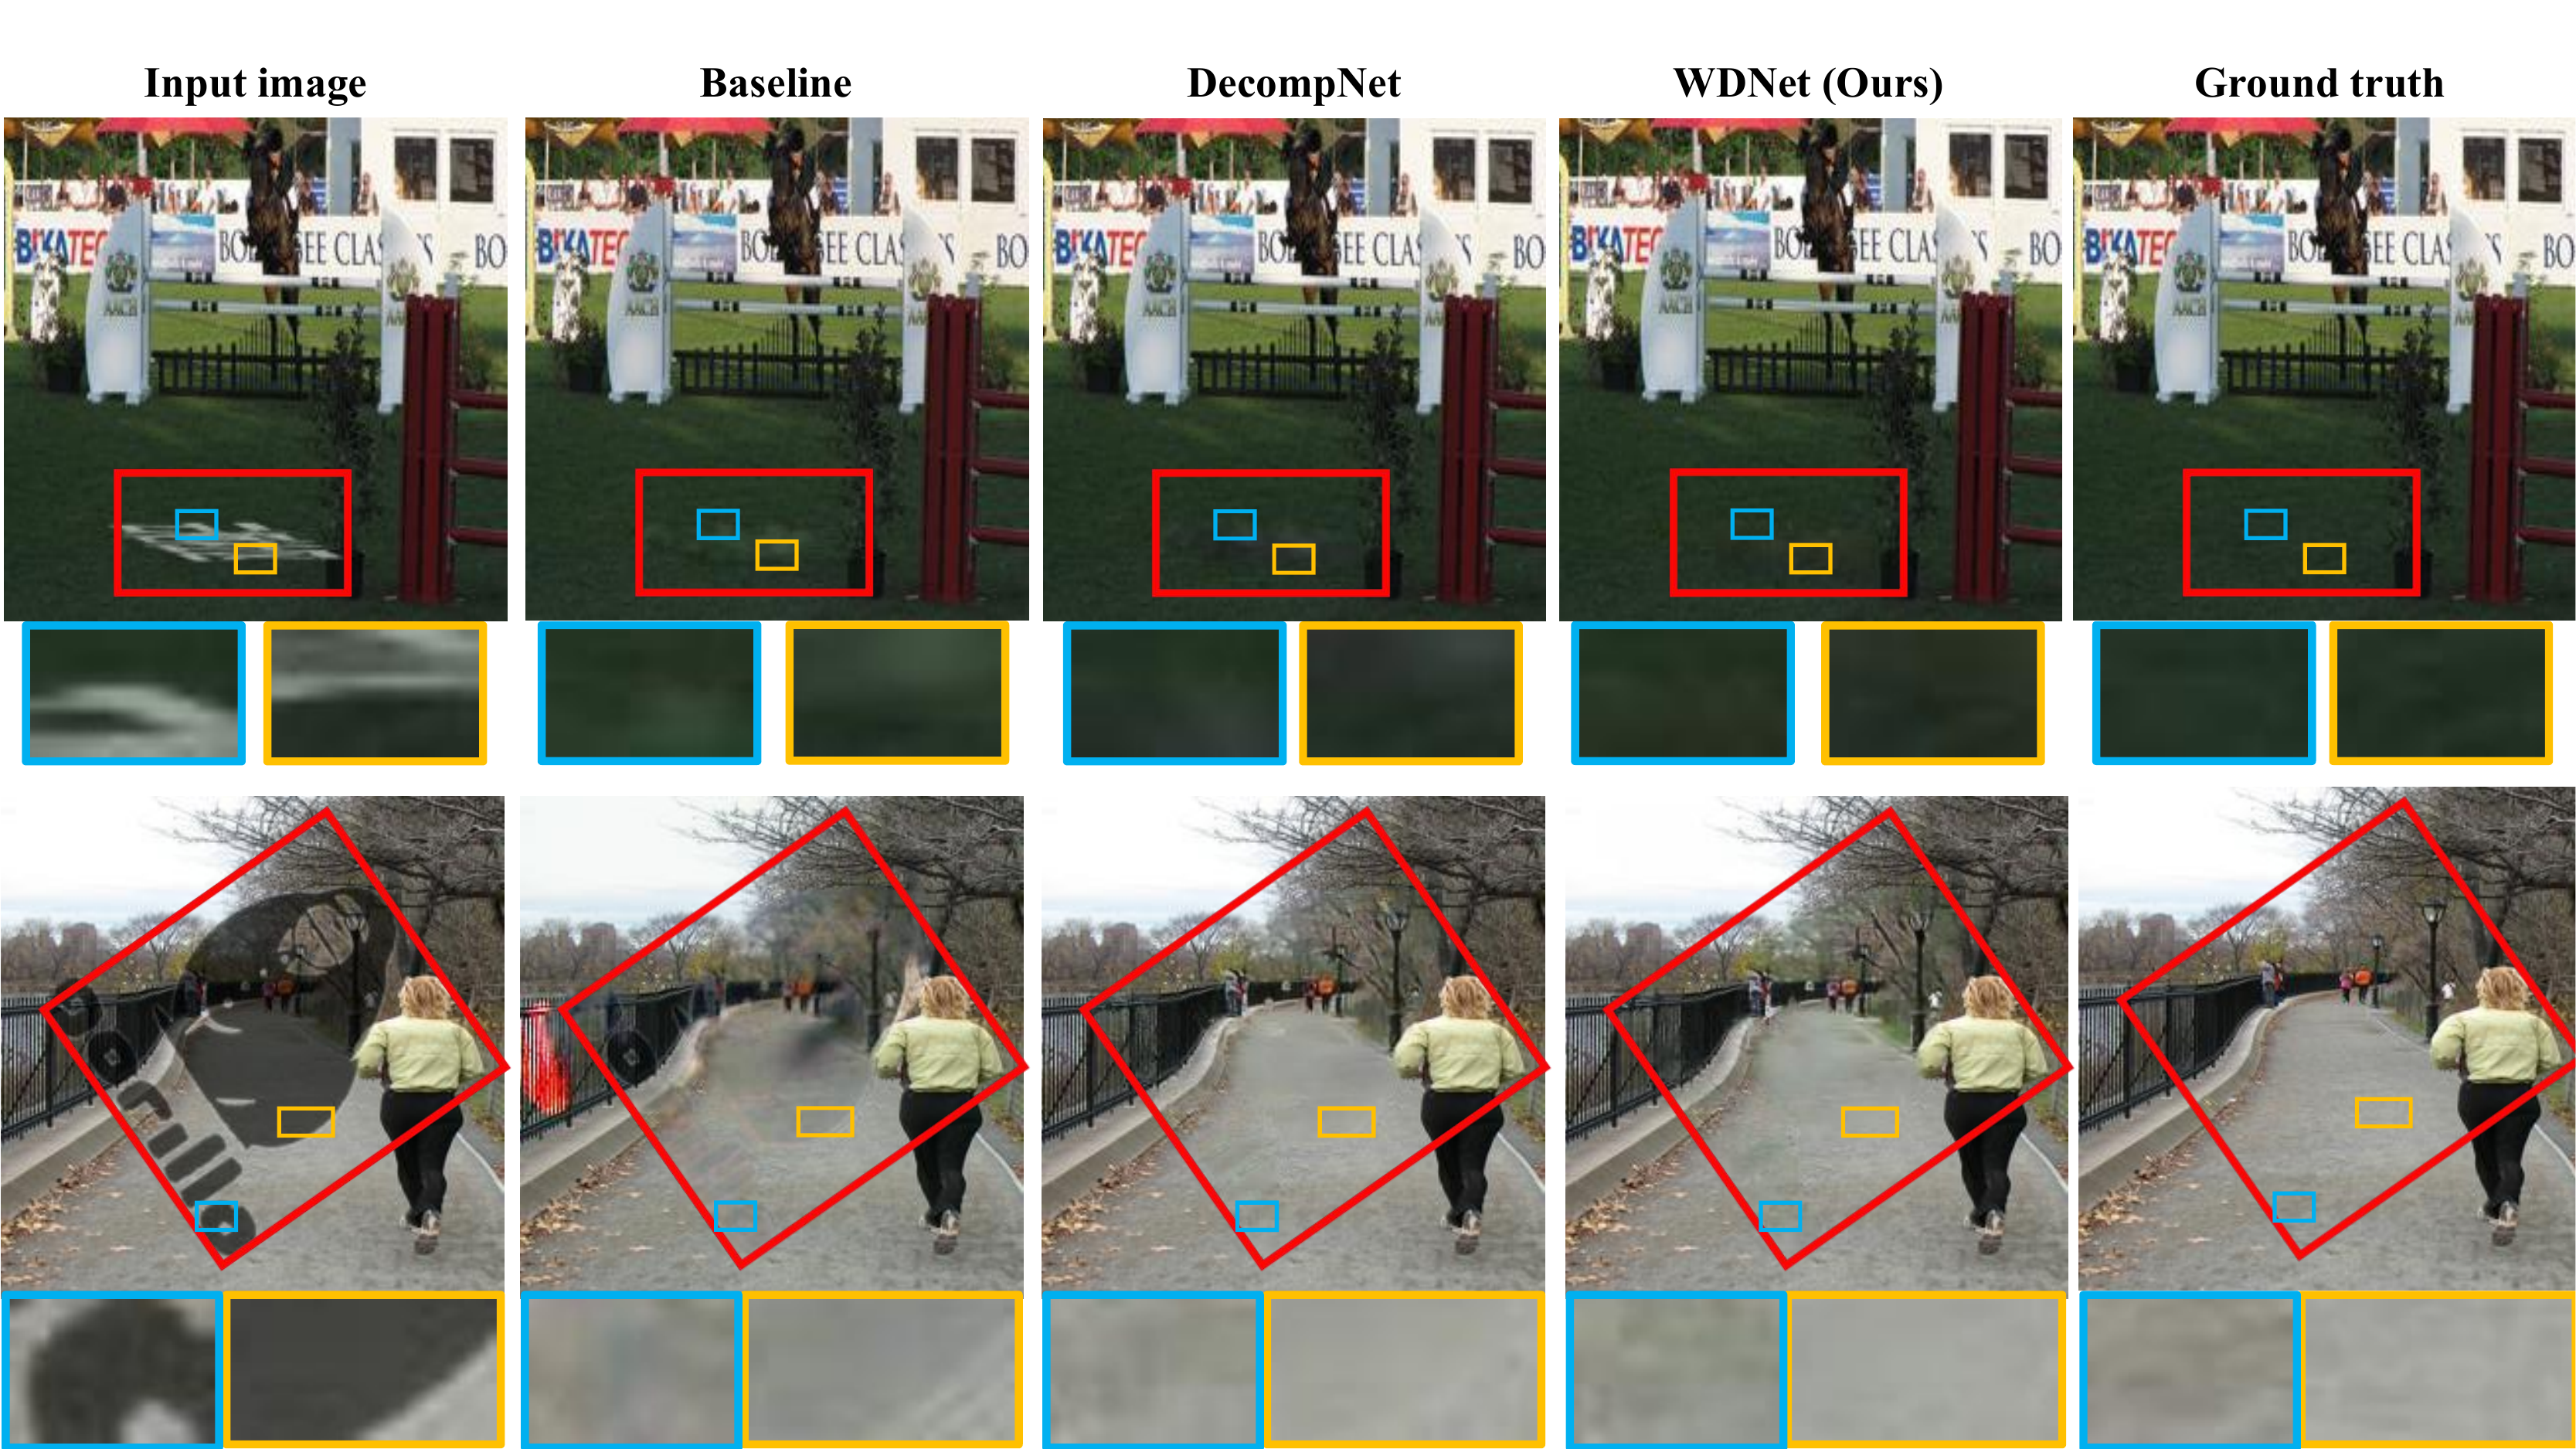}
\caption{Qualitative ablation comparisons on LVW (the first row) and CLWD (the second row) datasets. }
%\caption{Qualitative comparisons with state-of-the-art on some images from LVW and CLWD. The watermarks is the results of WDNet.}
%\caption{Trade-off between efficiency and accuracy for some existing methods and the proposed super-BPD. Based on the region F-measure~\cite{pont2016supervised}, super-BPD achieves competing performance while being near real-time on the PASCAL Context Dataset~\cite{mottaghi2014role}.}
\label{fig:sup_ablation_study_clwd}
\centering
\end{figure*}
