# Supplementary material for: WDNet: Watermark-Decomposition Network for Visible Watermark Removal
Source: arXiv:2012.07616 source file (2020-12-15)
Supplement: Supplementary file 4 [file tab_sup_loss_weight.tex]

\begin{table}[!h]
\small

\begin{center}
\begin{tabular}{c|c|c|c|c}
\toprule[1pt]
$\lambda_1$        &1   & 10    &50        & 100\\ \hline
$\mathrm{RMSE}_w$        & 19.58 & 18.36  & \bf{17.49} & 17.92\\  
\midrule[1pt]
$\lambda_2$        &1e-3   & 1e-2    &1e-1        & 1\\ \hline
$\mathrm{RMSE}_w$        & 19.01 & \bf{17.49}  &18.09  &18.23 \\  
\midrule[1pt]
$\lambda_3$        &1   & 10    &50        & 100\\ \hline
$\mathrm{RMSE}_w$        & 18.33 & \bf{17.49}  & 18.17 & 18.42\\  
\midrule[1pt]
$\lambda_4$        &1   & 10    &50        & 100\\ \hline
$\mathrm{RMSE}_w$        & 18.49 & \bf{17.49}  & 18.64 &19.82 \\  
\bottomrule[1pt]
\end{tabular}
\end{center}
%\vspace{-1mm}
\caption{Effects of four Loss weights on the performance $\mathrm{RMSE}_w$.}
\label{tab:sup_influenceoflossweights}
%\vspace{-4mm}
\end{table}
